# Supplementary material for: Low energy band structure and symmetries of UTe2 from angle resolved photoemission spectroscopy
Source: arXiv:1911.10152 ancillary file (2019-11-22)
Supplement: Supplementary file 1 [file SI_UTe2_1121_min.pdf]

*Supplemental Material for*

# Low energy band structure and symmetries of $UTe_2$ from angle resolved photoemission spectroscopy

Lin Miao[1,*], Shouzheng Liu[2,*], Yishuai Xu[2], Erica Kotta[2], Chang-Jong Kang[3], Sheng Ran[4,5], Johnpierre Paglione[5], Gabriel Kotliar[3], Nicholas P. Butch[4,5], Jonathan D. Denlinger[6,†], and L. Andrew Wray[2,‡]

1. School of Physics, Southeast University, Nanjing 211189, China.
2. Department of Physics, New York University, New York, New York 10003, USA
3. Department of Physics and Astronomy, Rutgers University, Piscataway, NJ, 08854-8019, USA
4. NIST Center for Neutron Research, National Institute of Standards and Technology, 100 Bureau Drive, Gaithersburg, MD 20899, USA
5. Quantum Materials Center, Department of Physics, University of Maryland, College Park, MD 20742, USA
6. Advanced Light Source, Lawrence Berkeley National Laboratory, Berkeley, CA 94720, USA

[*] These authors contributed equally to this work

[†] Email: jddenlinger@lbl.gov

[‡] Email: lawray@nyu.edu

## Note 1: Evaluation of Fermi nesting by joint density of states (JDOS)

The rectangular Fermi surface imaged in main text Fig. 2(a) is suggestive of strong Fermi surface nesting, raising the question of why the material does not have density wave order. To evaluate this, we have performed joint density of states (JDOS) convolutions [1-4], which correspond roughly with the quasiparticle interference images obtained by scanning tunneling microscopy, and provide a means to identify density wave instabilities. The JDOS amplitude is defined as N(q) = $\Sigma_k A(E_f,k)*A(E_f,k+q)$ where the $A(E_f,k)$ is the Fermi surface density of states. Indeed, using the main text Fig. 2(a) Fermi surface as the template for $A(E_f,k)$ results in a JDOS convolution that shows an extremely strong column-like peak at the $k_x$ Brillouin zone boundary (Fig. S6(a-b)), suggestive of near-neighbor antiferromagnetic correlations along the uranium chain. No analogous feature is visible near the $k_y$ Brillouin zone boundary, as the large velocity of the Te band results in very little density of states at the Fermi level.

However, the appearance of strong nesting is misleading, both because it neglects the significant 3D dispersion identified in the main text Fig. 3(a), and because focusing on the main text Fig. 2(a) Fermi surface excludes the heavy Z-point band. Factoring in the 3D dispersion via a parabolic fit of the two light bands ([Fig. S7) yields a corrected JDOS convolution with only a very weak feature at the Brillouin zone boundary (see Fig. S6(c)). Adding in the heavy Z-point band contributes strong short-wavelength scattering channels, and causes the nesting-associated local maximum to vanish altogether (see Fig. S6(a), red curve). The tendency towards antiferromagnetism along the uranium chain axis is further suppressed by the fact that diagonally coordinated chains are offset by half a unit cell along the x-axis, causing the interchain coupling to be frustrated in this scenario (see Fig. S6(d) diagram). Nonetheless, nesting of the light uranium band will support spin fluctuations that may facilitate Cooper pairing.

## Note 2: Fitting of 3D bands' dispersion

The JDOS evaluation is based on the spectra of 3D fitted band structure as shown in Fig. S8, which has involved two procedures: (i) The fitting of electronic band dispersion near the Fermi level as shown in the Fig.S7 and (ii) To apply a Lorentzian broadening to the fitted band dispersion, as described below.

For the quasi-1D uranium band which is normal to $k_x$-axis, the intensity distribution is given by:

$$I_U(k_x,k_y,k_z) = A(k_y,k_z) * \frac{w}{w^2+(k_x-x_c)^2}. \quad (1)$$

In the equation, $A(k_y,k_z)$ is proportional to $1/|\nabla_k E|$, which reflects the Fermi level density of states, and can be calculated from the fitted equation. Also once are $k_y$,$k_z$

given, one can also calculate from the fitted band dispersion where the band locates on $k_x$ axis, $x_c$. $w$ is the FWHM for the Lorentzian broadening distribution, is set to be 0.14Å$^{-1}$.

The impact of the quasi-1D tellurium band to the JDOS is neglectable. It is treated same as uranium band, except that its intensity broadening is along $k_y$-axis. The band dispersion equation is roughly estimated as E=2.2eV- 16.2eV(Å)$^2$$k_y^2$. The intensity of the tellurium band is nearly invisible in Fig.S8(c-d) due to its weak intensity, as a result of the large Fermi velocity of tellurium band.

As for isotropic heavy Z-point electron pocket, the intensity distribution is given by:

$$I(k_x, k_y, k_z) = A * \frac{w}{w^2+|\vec{k}-\vec{r_z}|^2}, \qquad (2)$$

$A$ is a constant to describe the Z-point pocket intensity. $\vec{r_z}$ is where Z point locates, and $w$ is set to be 0.229Å$^{-1}$, which is the radius for Z-point electron pocket acquired by fitting.

**Reference:**


[1] J. E. Hoffman, K. McElroy, D.-H. Lee, K. M Lang, H. Eisaki, S. Uchida, and J. C. Davis. Imaging quasiparticle interference in $Bi_2Sr_2CaCu_2O_{8+\delta}$. Science **297**, 1148–1151 (2002).

[2] Q.-H. Wang, and D.-H. Lee, Quasiparticle scattering interference in high-temperature superconductors. Phys. Rev. B **67**, 20511 (2003).

[3] R. S. Markiewicz, Bridging k and q space in the cuprates: comparing angle-resolved photoemission and STM results. Phys. Rev. B **69**, 214517 (2004).

[4] K. McElroy, G.-H. Gweon, S. Y. Zhou, J. Graf, S. Uchida, H. Eisaki, H. Takagi, T. Sasagawa, D.-H. Lee, and A. Lanzara, Elastic scattering susceptibility of the high temperature superconductor $Bi_2Sr_2CaCu_2O_{8+\delta}$: a comparison between real and momentum space photoemission spectroscopies. Phys. Rev. Lett. **96**, 067005 (2006).

[5] Y. Xu, Y. Sheng, and Y.-F. Yang, Phys. Rev. Lett. 123, 217002 (2019)..

**Fig. S1**

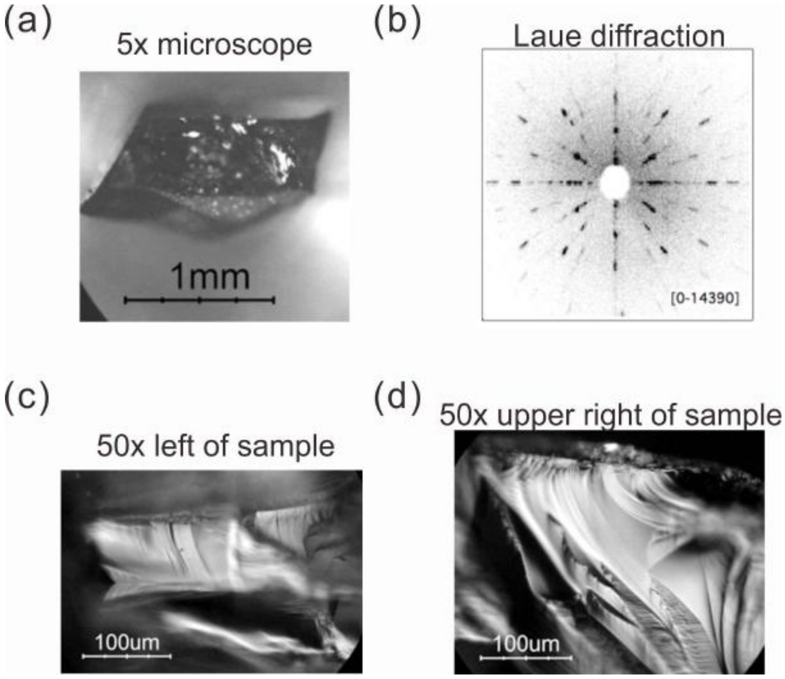


**Fig. S1. The characterization of cleaved $UTe_2$**. (a) The cleaved sample surface under 5x microscope. (b) Normal incidence X-ray Laue diffraction from the cleaved $UTe_2$ sample indicating a (001) cleavage orientation. Most samples cleaved along other orientations, resulting in non-(001) Laue patterns (not shown; such samples were excluded from this study). (c) The zoom-in (x50) image of a shiny and relatively flat area at the left part of $UTe_2$ sample. (d) A larger shiny flat area at the upper right part of $UTe_2$ sample, where the ARPES measurements were taken.

**Fig. S2**

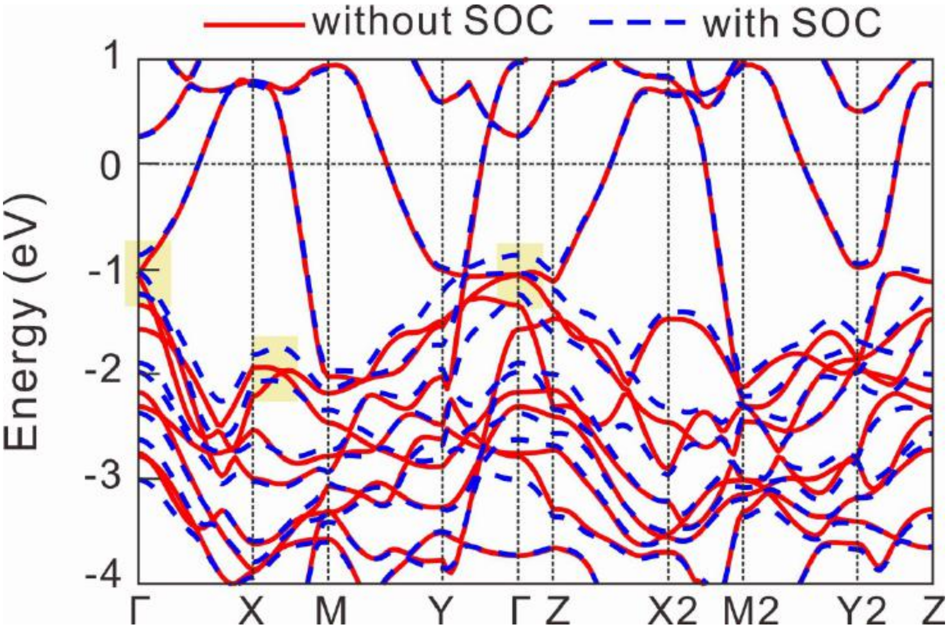


**Fig. S2. The comparison of $ThTe_2$ DFT without spin-orbital coupling (red lines) and with (blue dashed lines).** The inclusion of SOC in the DFT calculations lifts degeneracies at some points (shaded in the yellow). However, the impact of SOC is minimal near the Fermi level in these calculations.

**Fig. S3**

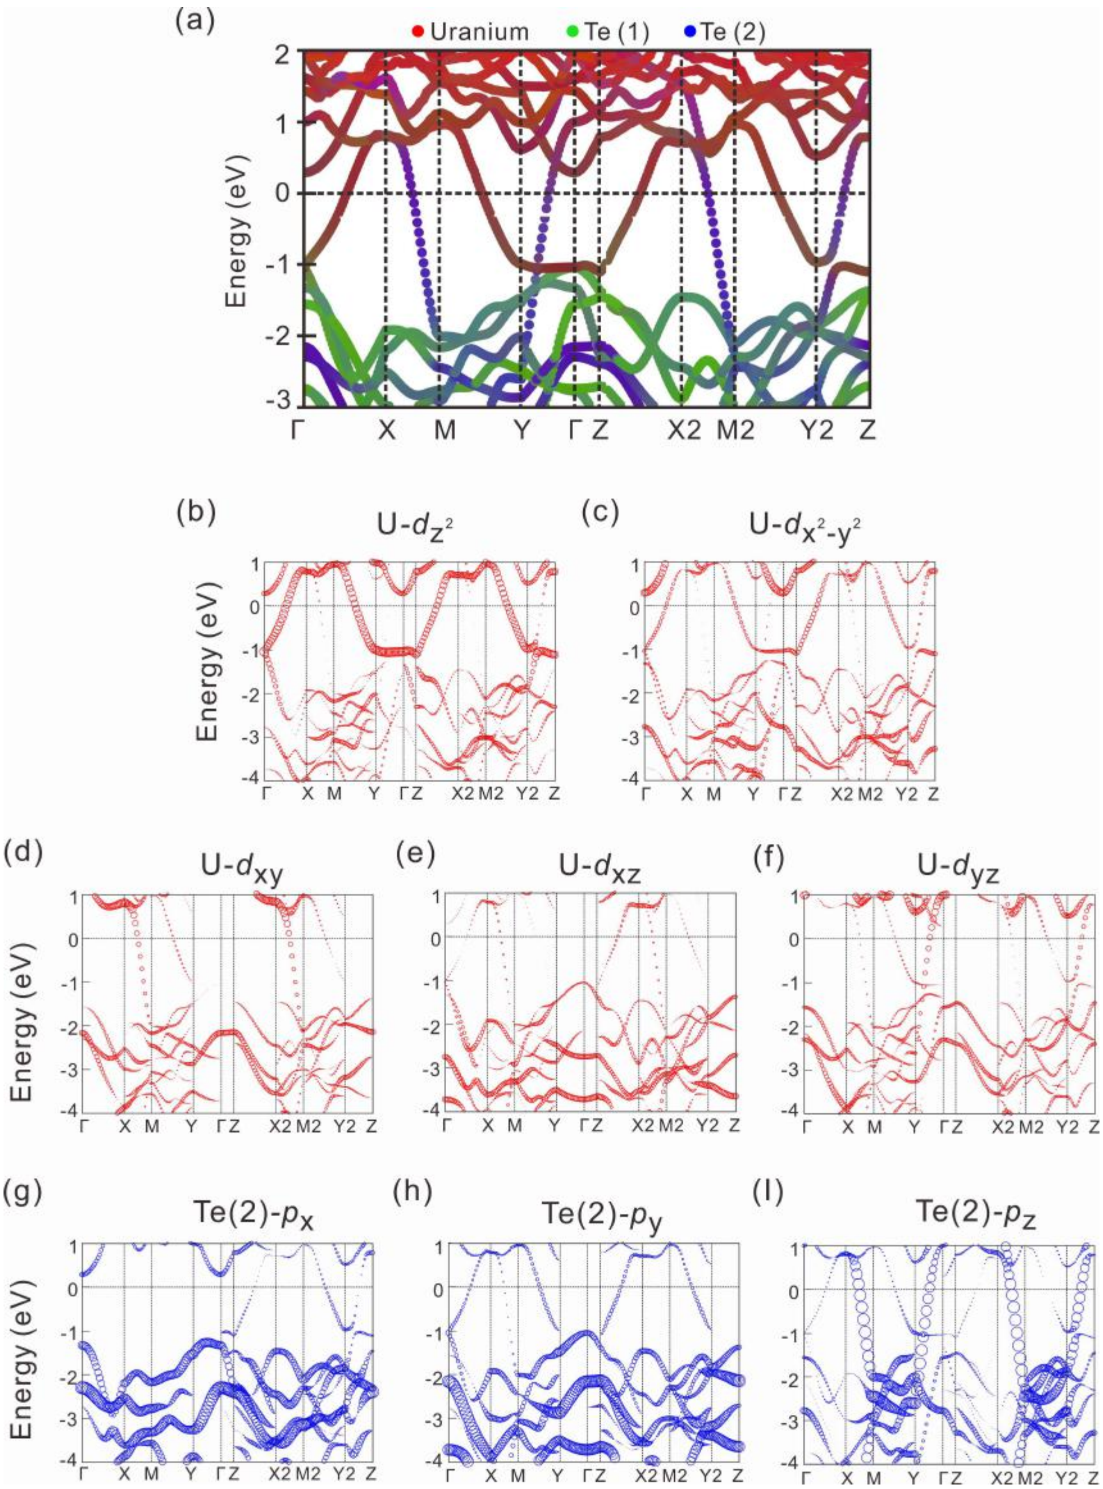


**Fig. S3. The orbital-resolved partial density of states from $ThTe_2$ DFT.** (a) The atomic sites-resolved DFT-calculated band structure of $UTe_2$. It is plotted with a rectangle path in the Brillouin zone (main text Fig.1(b)). The RGB color system is used to

represent the density of states at the atomic sites, e.g. uranium is noted with red, Te(1) is noted with green, Te(2) is noted with blue. (b-f) The PDOS of different 6*d*-orbital symmetries for uranium sites are shown, revealing large $6d_{z2}$ character in the Γ-X dispersive band. (g-i) The PDOS within tellurium 5*p* orbitals for the Te(2) sites, revealing the Γ-Y dispersive band to have large $5p_z$ character.

**Fig. S4**

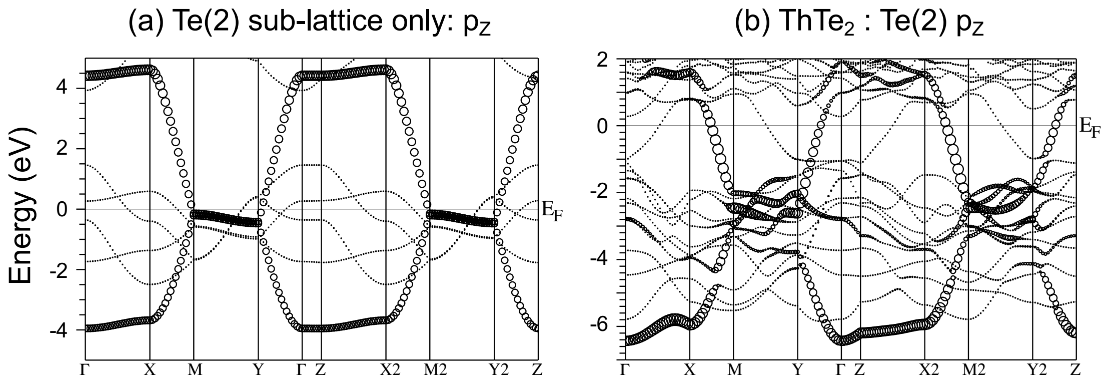


**Fig. S4. Te(2) linear chain electronic structure.** (a) The band structure of the Te(2) site planar sublattice reveals a large 8 eV bonding-antibonding splitting of the $p_z$ orbitals resulting from the small ≈*b*/2=3.1 Å near-neighbor distance along y-axis linear chains. (b) The large Te(2) bonding-antibonding splitting relative to other Te(2) or Te(1) p-orbital bands enables the existence of the hole-like 1D Fermi surface sheets with large band velocity in $ThTe_2$.

**Fig. S5**

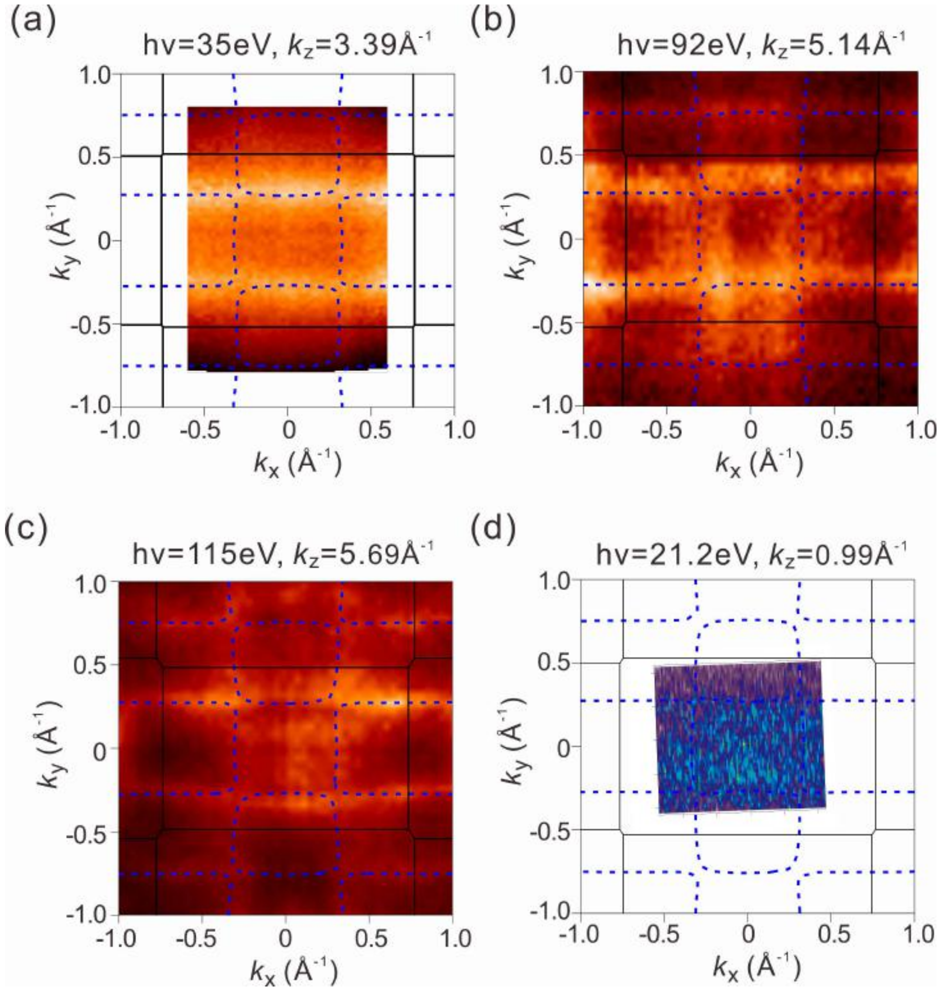


**Fig. S5. The Fermi surface of $UTe_2$ under different incident photon energies.** Rapid scans of the Fermi surface were performed with photon energy of (a) hv=35eV, (b) hv=92eV, (c) hv=115eV and (d) hv=21.2eV, and overlaid with the Fermi surface from $ThTe_2$ DFT.

## Fig. S6

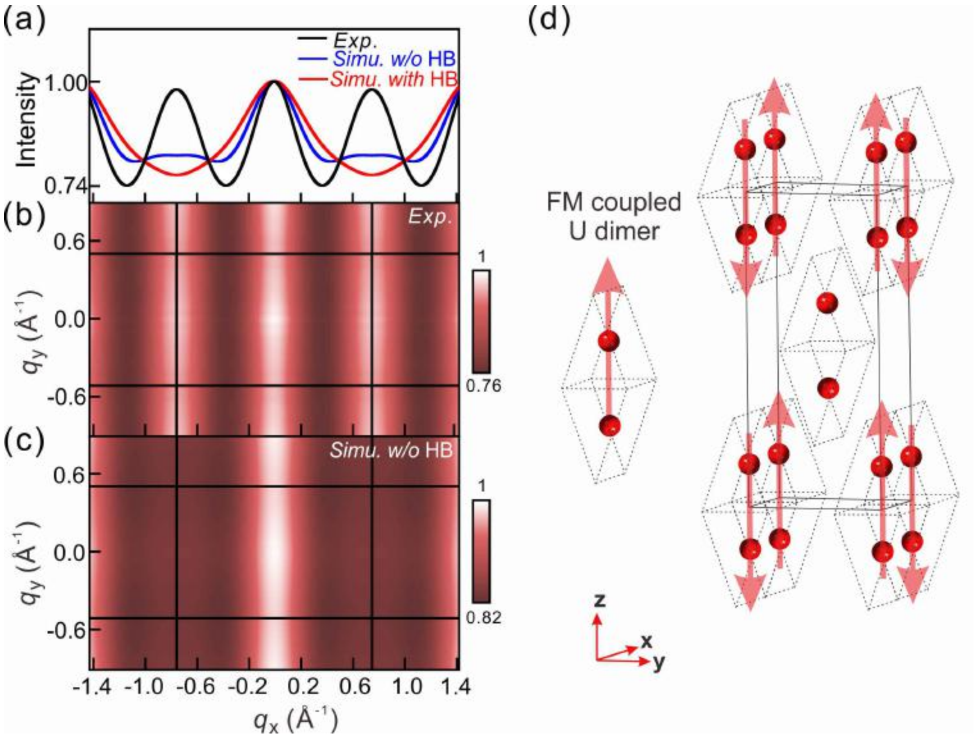


**Fig. S6. Weak Fermi surface nesting.** (a) Nesting JDOS curves averaged over $q_y$ are obtained from (black) the main text Fig. 2(a) $k_x - k_y$ Fermi surface, (blue) a 3D-fitted band structure neglecting the Z-point heavy electron band (HB), and (red) the fitted band structure incorporating the heavy Z-point band. The octagonal Brillouin zone is simplified to a rectangle, due to the limited range of the main text Fig. 2(a) template. (b-c) Full $q_x - q_y$ plane results of (b) the main text Fig. 2(a) experimental data convolution and (c) the fitted band structure convolution. (d) A diagram shows an antiferromagnetic structure previously considered in previous DMFT numerics [5], in which magnetic coupling to the central uranium dimer chain is geometrically frustrated.

**Fig. S7**

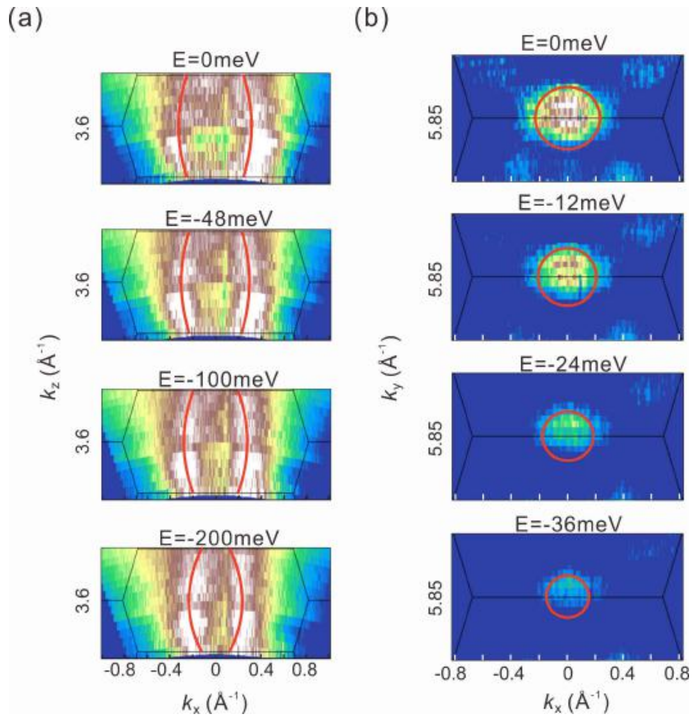


**Fig. S7. The fitting of uranium light and heavy band pockets** (a) The fitting of uranium light band by using equation $E=0.416eV*(-1+k_x^2/a+ k_y^2/b+ k_z^2/c)$ where $a=0.313Å^{-1}$ (from fitting), $b=1.103$ $Å^{-1}$ (from DFT calculation) and $c=0.729$ $Å^{-1}$ (from fitting). (b) The fitting of heavy band at z-point by using equation $E=0.061eV*(-1+k_x^2/0.229\ (Å^{-1})^2+ k_x^2/0.229(Å^{-1})^2+ k_z^2/0.229(Å^{-1})^2)$ with the assumption of an isotropic Fermi pocket.

**Fig. S8**

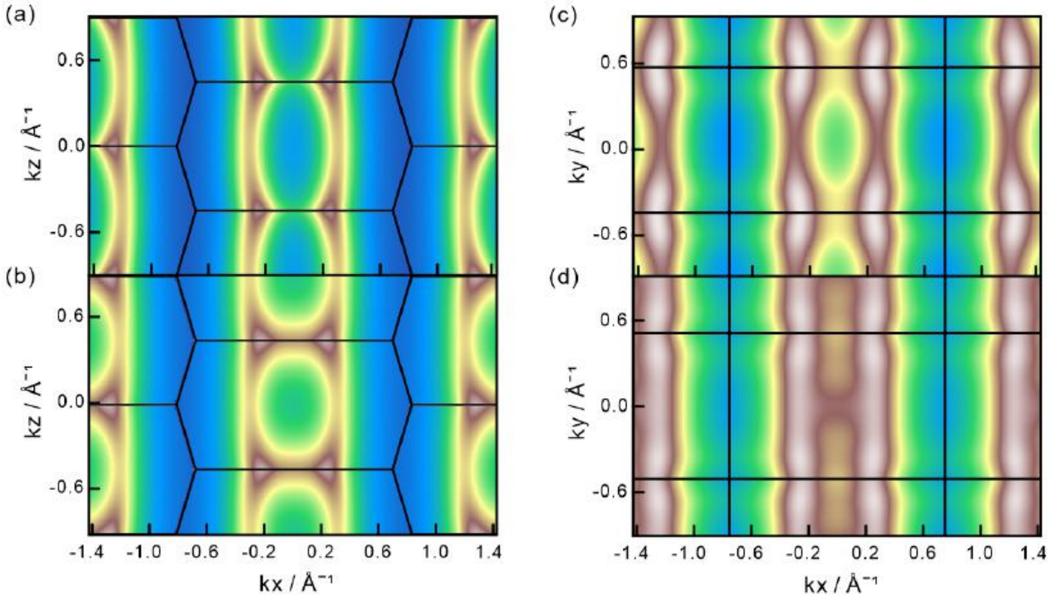


**Fig. S8. Simulated Fermi surface from fitted band equations** (a-b) Fitted uranium bands in $k_x$-$k_z$ plane ($k_y$=0) without (a) and with (b) the heavy Z-point electron pocket. The spectra are with $k_y$ integrated from -0.20$Å^{-1}$ to 0.20$Å^{-1}$. (c-d) Fitted uranium bands in $k_x$-$k_y$ plane ($k_z$=0.225 $Å^{-1}$) without (c) and with (d) heavy Z-point electron pocket. The spectra are with $k_z$ integrated from 0 to 0.45 $Å^{-1}$.
